# Supplementary material for: Markov models from the Square Root Approximation of the Fokker-Planck equation: calculating the grid-dependent flux
Source: arXiv:2010.03407 ancillary file (2020-11-13)
Supplement: Supplementary file 1 [file supplementary_material.pdf]

# Markov models from the Square Root Approximation of the Fokker-Planck equation: calculating the grid-dependent flux (Supplementary Material)

Luca Donati and Bettina G. Keller

*Department of Biology, Chemistry, Pharmacy,*

*Freie Universität Berlin, Takustraße 3, D-14195 Berlin, Germany**

Marcus Weber

*Zuse Institute Berlin, Takustr. 7, 14195 Berlin, Germany*

* luca.donati@fu-berlin.de

## I. ALGORITHM TO ESTIMATE THE ADJACENCY MATRIX

We provide an efficient algorithm to build the adjacency matrix when the $N_D$-dimensional state space of the system is discretized by a hyper-regular grid. The following MATLAB script, starting from a circulant matrix for periodic potentials or from a Toeplitz matrix for non-periodic potentials, exploits the Kronecker product to build iteratively the adjacency [1]. The function "krons(A,B)", which returns the Kronecker product of two sparse matrices A and B is taken from the package tensorlab 3.0 [2]

```
function A = adjacencyMatrix(Nbins, ND, option)
% Nbins  : number bins per each direction
% ND     : number of dimensions
% option : 'periodic' for periodic regular grid

v = zeros(1,Nbins);
v(2) = 1;

switch option
    case 'periodic'
        v(Nbins) = 1;
        A0 = sparse(circulant(v,1));
    otherwise
        A0 = sparse(toeplitz(v));
end

A = A0;
I2 = speye(Nbins);

for k = 1 : ND-1
    I1 = speye(size(A));                      % identity matrix
    A  = krons(A0, I1) + krons(I2, A);        % krons() from tensorlab
end
```

## II. ALGORITHM TO ESTIMATE THE RATE MATRIX USING THE RECTANGULAR METHOD

The following MATLAB script permits to construct efficiently the rate matrix **Q** of a system with a $N_D$-dimensional potential energy function, using the method "rectangular" for hyper-rectangular grids.

```
clear

% Number of dimensions of the system
ND        = 8;

% Diffusion
sigma     = 2.2;
beta      = 2/sigma^2;

% Potential energy function
V         = @(psi) (1 + cos(2 * psi));

% Grid per each dimension
Nbins     =  6;
xmin      = -pi;
xmax      =  pi;

x         = linspace(xmin, xmax, Nbins);
x(end)    = [];
dx        = x(2) - x(1);
Nbins     = Nbins - 1;

% Total number of microsets
N         = Nbins^ND;
```

```
% Hyper-rectangular grid
C     = {};

for jj = 1:ND
    C{jj} = x;
end

DX = cell(1,ND);
[DX{:}] = ndgrid(C{:});

% Adjacency matrix
A = adjacencyMatrix(Nbins, ND, 'periodic');

% Estimate potential on the grid
F = 0;
X = zeros(N,ND);
for jj=1:ND
    X(:,jj) = DX{jj}(:);
    F = F + V(X(:,jj));
end

% Flux
flux = sigma^2 / 2 / dx^2;
Af   = flux * A;

% SQRA
SQRA = sqrt(exp(- beta * F));
SQRA = SQRA / sum(SQRA);
```

```
% Diagonalization
D      = spdiags(SQRA, 0, N, N);
D1     = spdiags(1./SQRA, 0, N, N);
Q      = D1*Af*D;
Q      = Q + spdiags(- sum(Q,2), 0, N, N);

% Eigenspectrum
[evecs, evals] =  eigs(sparse(Q'), 2,'lr');
```

---


[1] Hiroki Sayama. Estimation of laplacian spectra of direct and strong product graphs. ArXiv, abs/1507.03030, 2016.

[2] N. Vervliet, O. Debals, L. Sorber, M. Van Barel, and L. De Lathauwer. Tensorlab 3.0, 2016. https://www.tensorlab.net.
